# Supplementary material for: Metric Distortion of Small-group Deliberation
Source: arXiv:2502.01380 source file (2026-08-13)
Supplement: Supplementary file 1 [file copeland_appendix.tex]

\section{Omitted Proofs from Section~\ref{sec:prelim}}
\label{app:omitted}

\subsection{Proof of \cref{lem1}}
Assume $d(W,X) = 1$. We have 
$$SC(W) - SC(X) = \sum_i \rho_i \left(d(i,W) - d(i,X) \right) = \sum_i \rho_i \phi_i = \E[D] = \gamma. $$
Next, by triangle inequality, $d(i,X) \ge d(X,W) - d(i,W)$, so that
$$ SC(X) = \sum_i \rho_i d(i,X) \ge \frac{1}{2} \sum_i \rho_i \left(d(X,W) - (d(i,W) - d(i,X) \right) = \frac{1}{2} \left(1 - \gamma \right). $$
Manipulating the above two inequalities completes the proof.

\subsection{Proof of \cref{thm:distort1}}

    Fix some metric $(d,\vec{\rho})$. Suppose the Copeland rule finds outcome $W$, and suppose $X$ is the social optimum. In the case where $W \succ X$, by the previous lemma, , the distortion is 
    $$\frac{SC(W)}{SC(X)} \le \frac{1 + \theta}{1-\theta}.$$ 
    Otherwise, there exists $Y$ such that $W \succ Y$ and $Y \succ X$. Then, the distortion is 
    $$ \frac{SC(W)}{SC(X)} = \frac{SC(W)}{SC(Y)} \cdot \frac{SC(Y)}{SC(X)} \le  \left( \frac{1 + \theta}{1-\theta}\right)^2. $$
    Since these bounds hold for all metrics $(d,\vec{\rho})$, the proof is complete.

\subsection{Proof of \cref{thm:lb_main}}
Consider an instance with two alternatives $W$ and $X$ that are distance $1$ unit apart on a line. Consider the distribution $D$ that yields the optimum solution to \cref{eq:opt}. Suppose $\Pr[D = a] = p_a$ for $a \in [-1,1]$. The we place voters of mass $p_a$ at distance $\frac{1+a}{2}$ from $W$ and $\frac{1-a}{2}$ from $X$.

First consider deterministic rules. Perturb $D$ slightly so that $p_k(W,X) = 1/2 + \delta$ for  $\delta \rightarrow 0$. Assume the social choice rule outputs $W$ in this case. Otherwise, perturb $D$ slightly so that $p_k(W,X) = 1/2 - \delta$, and the same rule will output $W$ as it is anonymous. As $\delta \rightarrow 0$, the distortion of this rules coincides with that of the rule that outputs $W$ in the former case. Now note that $SC(X) = \frac{1 - \E[D]}{2}$, and $SC(W) = \frac{1 + \E[D]}{2}$, which implies the distortion is at least  $\frac{1+\theta_k}{1-\theta_k}$.

Similarly, for randomized rules, suppose $W$ is output with probability $\alpha$. By perturbing $D$ slightly, $W$ will also be output with probability $1-\alpha$. Therefore, the  expected distortion is minimized when $\alpha = 1/2$, and is at least 
$\frac{1}{2} + \frac{1}{2} \cdot \frac{1+\theta_k}{1-\theta_k} = \frac{1}{1-\theta_k}.$
